# Supplementary material for: Teaching Unknown Objects by Leveraging Human Gaze and Augmented Reality in Human-Robot Interaction
Source: arXiv:2312.07638 source file (2023-12-12)
Supplement: Supplementary file 1 [file appendix.tex]

\begin{table*}[htb]
	\caption{Classification results of the 2D and 3D heatmap feature for different time window sizes (in ms), number of grid cells, and machine learning methods. The results are the average accuracy of a 5-fold cross validation. The best results per method are highlighted in bold.}
	\label{tbl:evalClassificationAppendix}
	\centering
	\begin{tabular}{ccr|cccccccccc}
		\toprule
		& &  & \multicolumn{10}{c}{Time window size (in ms)}\\
		Feature & ML & Grid & 50 & 100 & 150 & 200 & 250 & 300 & 350 & 400 & 450 & 500\\
		\midrule
		\multirow{30}{*}{\rotatebox{90}{2D heatmap}} & \multirow{10}{*}{\rotatebox{90}{\acs{KNN}}} & 5 & 68 & 70 & 73 & 78 & 78 & 80 & 79 & 80 & 81 & 80  \\
		& & 10 & 74 & 77 & 80 & 81 & 80 & 81 & 81 & 83 & 81 & 82  \\
		& & 15 & 76 & 79 & 81 & 80 & 82 & 82 & 82 & 84 & 84 & 84  \\
		& & 20 & 78 & 81 & 82 & 83 & 83 & 83 & 84 & 85 & 85 & 86  \\
		& & 25 & 78 & 82 & 83 & 84 & 84 & 84 & 84 & 85 & 85 & 85  \\
		& & 30 & 79 & 82 & 84 & 85 & 85 & 86 & 86 & 87 & 86 & 87  \\
		& & 35 & 80 & 83 & 85 & 85 & 86 & 85 & 86 & 87 & 86 & 87  \\
		& & 40 & 81 & 84 & 86 & 86 & 86 & 86 & 87 & 87 & 86 & 87  \\
		& & 45 & 82 & 85 & 86 & 87 & 86 & 86 & 87 & 87 & 86 & 87 \\
		& & 50 & 82 & 87 & 87 & 87 & 87 & 87 & \textbf{88} & \textbf{88} & 86 & \textbf{88}  \\ \cline{2-13}
		& \multirow{10}{*}{\rotatebox{90}{Bagged Trees}} & 5 & 79 & 82 & 83 & 84 & 84 & 84 & 85 & 85 & 86 & 86 \\
		& & 10 & 81 & 83 & 84 & 85 & 86 & 86 & 86 & 87 & 86 & 86 \\
		& & 15 & 82 & 84 & 85 & 85 & 86 & 86 & 86 & 87 & 87 & 86 \\
		& & 20 & 82 & 85 & 86 & 87 & 87 & 86 & 86 & 87 & 88 & 86 \\
		& & 25 & 83 & 86 & 86 & 87 & 87 & 87 & 86 & 87 & 88 & 86 \\
		& & 30 & 83 & 86 & 87 & 87 & 88 & 86 & 87 & 88 & 88 & 87 \\
		& & 35 & 84 & 86 & 87 & 88 & 87 & 88 & 87 & 88 & 87 & 87 \\
		& & 40 & 84 & 87 & 87 & 88 & 88 & 87 & 88 & \textbf{89} & 88 & 88  \\
		& & 45 & 84 & 87 & 88 & 88 & 88 & 88 & 87 & 88 & \textbf{89} & 88  \\
		& & 50 & 85 & 87 & 88 & 88 & \textbf{89} & 88 & 88 & 88 & \textbf{89} & 88 \\ \cline{2-13}
		& \multirow{10}{*}{\rotatebox{90}{Gaussian \acs{SVM}}} & 5 &73 & 78 & 80 & 81 & 82 & 82 & 82 & 83 & \textbf{84} & 82 \\
		& & 10 & 76 & 80 & 81 & 81 & 82 & 82 & 81 & 83 & 83 & 82 \\
		& & 15 & 78 & 80 & 81 & 81 & 82 & 82 & 81 & 82 & 83 & 82 \\
		& & 20 & 78 & 81 & 82 & 82 & 82 & 81 & 81 & 82 & 82 & 81 \\
		& & 25 & 78 & 80 & 81 & 81 & 81 & 80 & 80 & 81 & 81 & 80 \\
		& & 30 & 79 & 81 & 81 & 81 & 81 & 80 & 79 & 80 & 80 & 79 \\
		& & 35 & 79 & 80 & 80 & 81 & 80 & 79 & 78 & 78 & 78 & 76 \\
		& & 40 & 79 & 80 & 80 & 80 & 79 & 78 & 76 & 77 & 75 & 74 \\
		& & 45 & 79 & 80 & 80 & 79 & 78 & 77 & 74 & 75 & 74 & 73 \\
		& & 50 & 79 & 80 & 79 & 78 & 77 & 75 & 73 & 74 & 73 & 73 \\ \hline
		\multirow{30}{*}{\rotatebox{90}{3D heatmap}} & \multirow{10}{*}{\rotatebox{90}{\acs{KNN}}} & 5 & 73 & 79 & 79 & 81 & 81 & 80 & 81 & 82 & 82 & 82  \\
		& & 10 & 80 & 83 & 85 & 86 & 86 & 85 & 86 & 87 & 86 & 87 \\
		& & 15 & 82 & 87 & 87 & 88 & 88 & 88 & 88 & 88 & 88 & 88  \\
		& & 20 & 85 & 88 & 89 & 89 & 89 & 88 & 88 & 88 & 87 & 88  \\
		& & 25 & 87 & 89 & 90 & 90 & 90 & 88 & 89 & 89 & 89 & 89 \\
		& & 30 & 88 & 90 & 90 & 91 & 90 & 89 & 88 & 89 & 88 & 89 \\
		& & 35 & 89 & 91 & 91 & 91 & 90 & 89 & 89 & 89 & 88 & 89 \\
		& & 40 & 90 & \textbf{92} & 91 & 90 & 90 & 90 & 89 & 89 & 88 & 89  \\
		& & 45 & 91 & \textbf{92} & \textbf{92} & 91 & 89 & 89 & 88 & 89 & 88 & 88  \\
		& & 50 & 91 & \textbf{92} & \textbf{92} & 91 & 90 & 89 & 89 & 89 & 88 & 89 \\ \cline{2-13}
		& \multirow{10}{*}{\rotatebox{90}{Bagged Trees}} & 5 & 80 & 83 & 84 & 86 & 86 & 86 & 85 & 87 & 87 & 86  \\
		& & 10 & 84 & 86 & 87 & 87 & 88 & 88 & 87 & 88 & 88 & 87  \\
		& & 15 & 84 & 87 & 88 & 87 & \textbf{89} & 88 & 87 & \textbf{89} & 88 & 88 \\
		& & 20 & 85 & 87 & 88 & 88 & 88 & 87 & 88 & 87 & 87 & 88  \\
		& & 25 & 86 & 87 & 88 & 88 & 88 & 87 & 87 & 87 & 86 & 86 \\
		& & 30 & 86 & 87 & 88 & 88 & 88 & 87 & 87 & 87 & 86 & 87 \\
		& & 35 & 87 & 88 & 88 & 88 & 87 & 87 & 87 & 87 & 87 & 86 \\
		& & 40 & 87 & 88 & 88 & 88 & 87 & 87 & 87 & 87 & 86 & 86 \\
		& & 45 & 87 & 88 & 88 & 88 & 87 & 87 & 87 & 86 & 86 & 85 \\
		& & 50 & 87 & 88 & 88 & 87 & 86 & 86 & 86 & 85 & 86 & 84  \\ \cline{2-13}
		& \multirow{10}{*}{\rotatebox{90}{Gaussian \acs{SVM}}} & 5 & 75 & 79 & 80 & 81 & 81 & 82 & 82 & \textbf{83} & \textbf{83} & 82 \\
		& & 10 & 79 & 81 & 82 & \textbf{83} & 82 & 81 & 81 & 81 & 81 & 80 \\
		& & 15 & 80 & 82 & 82 & 80 & 80 & 79 & 77 & 78 & 77 & 76 \\
		& & 20 & 81 & 81 & 80 & 78 & 77 & 76 & 74 & 75 & 75 & 74  \\
		& & 25 & 81 & 80 & 78 & 76 & 75 & 74 & 72 & 74 & 73 & 73 \\
		& & 30 & 81 & 79 & 77 & 75 & 74 & 73 & 72 & 73 & 73 & 73 \\
		& & 35 & 81 & 78 & 76 & 74 & 73 & 73 & 72 & 73 & 73 & 73 \\
		& & 40 & 80 & 77 & 74 & 73 & 73 & 72 & 72 & 73 & 73 & 73 \\
		& & 45 & 80 & 76 & 74 & 73 & 73 & 73 & 72 & 73 & 73 & 73 \\
		& & 50 & 79 & 75 & 73 & 73 & 73 & 72 & 72 & 73 & 73 & 73 \\ \hline
	\end{tabular}
\end{table*}

\begin{table*}[htb]
	\caption{Regression error results as the average absolute error ($\cdot 10^{2}$) of a 5-fold cross validation, normalized to the image resolution. The columns X and Y denote the position of the bounding box, W is the width, and H is the height of the bounding box. The best values per method are highlighted in bold.}
	\label{tbl:evalRegressionAppendix}
	\centering
	
    \setlength\tabcolsep{4.5pt}
	\begin{tabular}{ccc|cccc|cccc|cccc|cccc|cccc}
		\toprule
		&  &  & \multicolumn{20}{c}{Time window size (in ms)}\\
		Feat. & ML & Grid & \multicolumn{4}{c}{100} & \multicolumn{4}{c}{200} & \multicolumn{4}{c}{300} & \multicolumn{4}{c}{400} & \multicolumn{4}{c}{500}\\
		& & & X & Y & W & H & X & Y & W & H & X & Y & W & H & X & Y & W & H & X & Y & W & H\\
		\midrule
		\multirow{30}{*}{\rotatebox{90}{2D heatmap}} & \multirow{10}{*}{\rotatebox{90}{Gaussian Process}} & 5 & 7.0 & 8.0 & 13.8 & 16.4 & 7.2 & 7.9 & 13.4 & 16.1 & 7.7 & 8.2 & 13.9 & 16.1 & 7.8 & 8.0 & 13.7 & 16.1 & 8.8 & 7.3 & 13.4 & 16.3 \\
		& & 10 & \textbf{6.1} & \textbf{6.8} & 13.0 & 15.3 & 6.5 & 6.9 & 12.5 & 15.2 & 8.8 & 7.5 & 13.8 & 15.3 & 8.1 & 7.1 & 13.2 & 16.5 & 8.2 & 6.9 & 13.8 & 15.5 \\
		& & 15 & \textbf{6.1} & \textbf{6.8} & 12.7 & 15.3 & 7.8 & 9.5 & 13.5 & 16.8 & 9.4 & 8.4 & 14.3 & 15.7 & 8.3 & 7.7 & 12.4 & 15.8 & 8.4 & 7.1 & 13.7 & 15.8 \\
		& & 20 & 6.2 & 6.9 & 12.9 & 15.3 & 8.8 & 10.2 & 14.1 & 17.0 & 9.4 & 9.9 & 13.7 & 16.3 & 8.1 & 7.6 & 12.4 & 15.4 & 8.5 & 8.5 & 13.2 & 17.5 \\
		& & 25 & 6.8 & \textbf{6.8} & 12.7 & 15.2 & 8.8 & 8.8 & 13.9 & 16.8 & 9.3 & 9.2 & 14.3 & 15.9 & 8.4 & 8.9 & 13.0 & 15.8 & 8.5 & 8.5 & 13.4 & 17.0 \\
		& & 30 & 8.6 & \textbf{6.8} & 12.9 & 15.4 & 8.8 & 10.8 & 14.0 & 17.3 & 9.3 & 11.1 & 14.3 & 17.7 & 8.7 & 10.6 & 14.1 & 17.3 & 8.9 & 8.6 & 13.7 & 17.5 \\
		& & 35 & 7.9 & \textbf{6.8} & 12.7 & \textbf{15.1} & 8.8 & 10.8 & 13.4 & 17.3 & 9.3 & 11.1 & 14.3 & 17.7 & 8.7 & 10.6 & 14.1 & 17.3 & 8.6 & 8.6 & 13.9 & 17.5 \\
		& & 40 & 8.1 & \textbf{6.8} & \textbf{12.2} & 16.4 & 9.1 & 10.8 & 12.7 & 17.3 & 9.3 & 11.1 & 14.3 & 17.7 & 8.7 & 10.6 & 14.1 & 17.3 & 8.6 & 10.3 & 13.8 & 17.5 \\
		& & 45 & 8.1 & \textbf{6.8} & 12.6 & 16.9 & 9.1 & 10.8 & 14.2 & 17.3 & 9.3 & 11.1 & 14.3 & 17.7 & 8.7 & 10.6 & 14.1 & 17.3 & 9.1 & 10.3 & 14.4 & 17.5 \\
		& & 50 & 8.0 & \textbf{6.8} & 12.6 & 16.8 & 9.1 & 10.8 & 14.2 & 17.3 & 9.3 & 11.1 & 14.3 & 17.7 & 8.7 & 10.6 & 14.1 & 17.3 & 9.1 & 10.3 & 14.4 & 17.5 \\ \cline{2-23}
		& \multirow{10}{*}{\rotatebox{90}{Bagged Trees}} & 5 & 7.0 & 7.9 & 13.5 & 16.4 & 7.2 & 7.7 & 13.2 & 16.3 & 7.6 & 8.1 & 13.4 & 16.1 & 7.4 & 7.8 & 13.5 & 15.7 & 7.8 & 7.3 & 13.6 & 15.7 \\
		& & 10 & \textbf{6.4} & 7.0 & 13.0 & 15.3 & 6.7 & 7.1 & 12.6 & 15.2 & 7.4 & 7.9 & 12.5 & 15.3 & 7.0 & 7.7 & 12.5 & 14.9 & 7.4 & 7.3 & 12.5 & 15.0\\
		& & 15 & \textbf{6.4} & 7.1 & 12.6 & 15.1 & 6.8 & 7.3 & 12.3 & 14.9 & 7.5 & 8.0 & 12.5 & 15.3 & 7.2 & 7.9 & \textbf{12.0} & 15.0 & 7.8 & 7.2 & 12.2 & 15.1 \\
		& & 20 & \textbf{6.4} & \textbf{6.9}& 12.7 & 14.8 & 6.9 & 7.1 & 12.2 & 14.8 & 7.6 & 8.0 & 12.2 & 15.4 & 7.1 & 7.8 & 12.2 & 15.0 & 7.7 & 7.2 & 12.1 & 14.9 \\
		& & 25 & 6.5 & 7.0 & 12.6 & 14.8 & 7.1 & 7.4 & 12.2 & 14.7 & 7.7 & 8.2 & 12.1 & 14.8 & 7.2 & 7.9 & 12.1 & 14.6 & 7.7 & 7.4 & \textbf{12.0}  & 14.7 \\
		& & 30 & 6.5 & \textbf{6.9} & 12.4 & 14.7 & 6.9 & 7.3 & 12.2 & 14.6 & 7.6 & 8.2 & 12.4 & 15.0 & 7.3 & 7.9 & 12.2 & 14.7 & 7.7 & 7.4 & 12.3 & 15.1 \\
		& & 35 & \textbf{6.4} & 7.0 & 12.2 & 14.5 & 7.1 & 7.3 & 12.1 & 14.4 & 7.6 & 8.2 & 12.1 & 14.8 & 7.3 & 7.9 & 12.1 & 14.4 & 7.8 & 7.5 & 12.1 & 14.7 \\
		& & 40 & 6.5 & 7.0 & 12.1 & \textbf{14.3}  & 7.1 & 7.3 & \textbf{12.0}  & 14.4 & 7.6 & 8.2 & \textbf{12.0}  & 14.5 & 7.4 & 8.0 & 12.1 & 14.6 & 7.8 & 7.4 & \textbf{12.0} & 14.4 \\
		& & 45 & 6.5 & 7.0 & 12.2 & 14.4 & 7.1 & 7.4 & 12.1 & 14.5 & 7.6 & 8.3 & 12.1 & 14.8 & 7.2 & 8.0 & \textbf{12.0}  & 14.5 & 7.6 & 7.6 & \textbf{12.0}  & 14.8 \\
		& & 50 & 6.6 & 7.1 & 12.3 & 14.4 & 7.1 & 7.4 & 12.2 & 14.4 & 7.6 & 8.3 & 12.3 & 14.5 & 7.3 & 8.1 & 12.1 & 14.6 & 7.8 & 7.5 & \textbf{12.0}  & 15.0 \\ \cline{2-23}
		& \multirow{10}{*}{\rotatebox{90}{Gaussian \acs{SVM}}} & 5 & 7.2 & 8.3 & 14.6 & 17.2 & 7.4 & 8.2 & 14.6 & 16.8 & 8.1 & 8.7 & 14.6 & 17.3 & 7.6 & 8.3 & 14.3 & 16.5 & 7.7 & 7.9 & 14.7 & 16.8\\
		& & 10 & 6.5 & 7.1 & 14.5 & 16.9 & 6.8 & 7.0 & 14.3 & 16.6 & 7.5 & 7.7 & 14.4 & 17.2 & 7.0 & 7.3 & 14.0 & 16.4 & 7.3 & 6.9 & 14.6 & 16.7\\
		& & 15 & \textbf{6.4}  & 7.0 & 14.4 & 16.6 & 6.9 & 7.0 & 13.9 & 16.2 & 7.6 & 7.8 & 14.0 & 16.7 & 7.1 & 7.4 & 13.8 & 16.0 & 7.5 & 7.1 & 14.2 & 16.1 \\
		& & 20 & 6.5 & 7.0 & 14.4 & 16.6 & 6.9 & 7.2 & 14.1 & 16.4 & 7.5 & 7.9 & 14.2 & 16.8 & 7.1 & 7.3 & 13.9 & 16.1 & 7.6 & 7.1 & 14.3 & 16.3 \\
		& & 25 & 6.5 & \textbf{6.9} & 14.0 & 16.4 & 7.0 & 7.2 & 13.8 & 16.0 & 7.6 & 7.8 & 13.9 & 16.5 & 7.2 & 7.6 & 13.8 & 15.8 & 7.7 & 7.2 & 14.1 & 15.9 \\
		& & 30 & 6.5 & \textbf{6.9} & 14.1 & 16.4 & 7.0 & 7.2 & 14.0 & 16.4 & 7.7 & 8.1 & 14.1 & 16.8 & 7.3 & 7.8 & 13.7 & 16.0 & 7.8 & 7.5 & 14.1 & 16.1 \\
		& & 35 & \textbf{6.4} & 7.0 & 13.7 & 16.0 & 7.0 & 7.2 & 13.7 & 15.8 & 7.7 & 8.0 & 13.7 & 16.1 & 7.3 & 7.8 & \textbf{13.4} & 15.6 & 7.7 & 7.4 & 13.7 & 15.7 \\
		& & 40 & 6.5 & 7.0 & 13.7 & 16.0 & 7.1 & 7.5 & 13.7 & 15.9 & 7.8 & 8.1 & 13.8 & 16.2 & 7.4 & 7.8 & 13.5 & \textbf{15.5} & 7.8 & 7.7 & 13.8 & 15.7 \\
		& & 45 & 6.6 & 7.0 & 13.9 & 16.3 & 7.1 & 7.4 & 13.8 & 16.0 & 7.8 & 8.3 & 14.0 & 16.6 & 7.5 & 8.0 & 13.7 & 16.0 & 7.9 & 7.7 & 14.1 & 16.2 \\
		& & 50 & 6.5 & 7.0 & 13.9 & 16.1 & 7.1 & 7.6 & 13.9 & 16.0 & 7.9 & 8.3 & 14.1 & 16.4 & 7.5 & 8.1 & 13.9 & 15.8 & 7.9 & 7.9 & 14.2 & 16.0 \\ \hline
		\multirow{30}{*}{\rotatebox{90}{3D heatmap}} & \multirow{10}{*}{\rotatebox{90}{Gaussian Process}} & 5 & 6.7 & 7.5 & 12.8 & 15.4 & 7.1 & 7.3 & 12.4 & 15.7 & 9.4 & 8.6 & 13.1 & 16.6 & 8.6 & 8.4 & 13.2 & 15.6 & 8.9 & 7.3 & 13.8 & 15.2 \\
		& & 10 & \textbf{5.8} & 6.2 & 11.4 & 12.9 & 7.6 & 7.6 & 12.2 & 16.8 & 9.3 & 11.1 & 14.3 & 17.7 & 8.7 & 10.6 & 14.1 & 17.3 & 8.9 & 8.6 & 12.9 & 17.5 \\
		& & 15 & 6.5 & \textbf{6.0} & 10.4 & \textbf{11.6} & 9.1 & 10.8 & 14.2 & 17.2 & 9.3 & 11.1 & 14.3 & 17.7 & 8.7 & 10.6 & 14.1 & 17.3 & 9.1 & 10.3 & 14.4 & 17.5 \\
		& & 20 & 7.4 & 8.3 & \textbf{9.9} & 16.3 & 9.1 & 10.8 & 14.2 & 17.3 & 9.3 & 11.1 & 14.3 & 17.7 & 8.7 & 10.6 & 14.1 & 17.3 & 9.1 & 10.3 & 14.4 & 17.5 \\
		& & 25 & 9.1 & 10.8 & 14.3 & 17.4 & 9.1 & 10.8 & 14.2 & 17.3 & 9.3 & 11.1 & 14.3 & 17.7 & 8.7 & 10.6 & 14.1 & 17.3 & 9.1 & 10.3 & 14.4 & 17.5 \\
		& & 30 & 9.1 & 10.8 & 14.3 & 17.4 & 9.1 & 10.8 & 14.2 & 17.3 & 9.3 & 11.1 & 14.3 & 17.7 & 8.7 & 10.6 & 14.1 & 17.3 & 9.1 & 10.3 & 14.4 & 17.5 \\
		& & 35 & 9.1 & 10.8 & 14.3 & 17.4 & 9.1 & 10.8 & 14.2 & 17.3 & 9.3 & 11.1 & 14.3 & 17.7 & 8.7 & 10.6 & 14.1 & 17.3 & 9.1 & 10.3 & 14.4 & 17.5 \\
		& & 40 & 9.1 & 10.8 & 14.3 & 17.4 & 9.1 & 10.8 & 14.2 & 17.3 & 9.3 & 11.1 & 14.3 & 17.7 & 8.7 & 10.6 & 14.1 & 17.3 & 9.1 & 10.3 & 14.4 & 17.5 \\
		& & 45 & 9.1 & 10.8 & 14.3 & 17.4 & 9.1 & 10.8 & 14.2 & 17.3 & 9.3 & 11.1 & 14.3 & 17.7 & 8.7 & 10.6 & 14.1 & 17.3 & 9.1 & 10.3 & 14.4 & 17.5 \\
		& & 50 & 9.1 & 10.8 & 14.3 & 17.4 & 9.1 & 10.8 & 14.2 & 17.3 & 9.3 & 11.1 & 14.3 & 17.7 & 8.7 & 10.6 & 14.1 & 17.3 & 9.1 & 10.3 & 14.4 & 17.5 \\ \cline{2-23}
		& \multirow{10}{*}{\rotatebox{90}{Bagged Trees}} & 5 & 6.7 & 7.4 & 12.7 & 15.2 & 7.1 & 7.5 & 12.3 & 15.0 & 7.9 & 7.9 & 12.5 & 15.2 & 7.6 & 7.7 & 12.5 & 15.0 & 7.8 & 7.5 & 12.6 & 15.2 \\
		& & 10 & \textbf{6.4} & \textbf{6.7} & 11.8 & 13.8 & 7.0 & 7.2 & 11.5 & 14.0 & 7.6 & 8.1 & 11.9 & 14.7 & 7.3 & 8.2 & 11.6 & 14.1 & 7.7 & 7.8 & 11.4 & 14.3\\
		& & 15 & \textbf{6.4} & 6.8 & 11.1 & 12.8 & 7.1 & 7.3 & 11.0 & 13.0 & 7.8 & 8.3 & 11.4 & 13.6 & 7.3 & 8.3 & 11.6 & 13.3 & 8.2 & 7.7 & 11.1 & 13.4 \\
		& & 20 & 6.7 & 7.0 & 11.0 & 12.7 & 7.2 & 7.3 & 11.0 & 13.1 & 7.9 & 8.2 & 11.1 & 13.4 & 7.5 & 8.2 & 11.2 & 13.5 & 8.1 & 7.8 & 10.9 & 13.6 \\
		& & 25 & 6.6 & 7.1 & 10.9 & 12.6 & 7.2 & 7.6 & 11.0 & 12.6 & 7.8 & 8.6 & 10.9 & 13.2 & 7.5 & 8.4 & 11.1 & 13.1 & 8.2 & 7.9 & 10.5 & 12.8\\
		& & 30 & 6.8 & 7.2 & 10.8 & \textbf{12.3} & 7.5 & 7.8 & 11.0 & 12.7 & 8.1 & 8.6 & 10.9 & 13.4 & 7.8 & 8.7 & 11.1 & 13.3 & 8.4 & 8.2 & 10.8 & 12.9 \\
		& & 35 & 7.0 & 7.3 & 11.0 & 13.0 & 7.4 & 7.8 & 11.2 & 13.1 & 8.1 & 8.7 & 11.0 & 13.8 & 7.7 & 8.6 & 11.0 & 13.8 & 8.3 & 8.2 & 10.8 & 13.3 \\
		& & 40 & 7.1 & 7.5 & 10.7 & 12.6 & 7.5 & 8.0 & 10.9 & 12.8 & 8.1 & 8.8 & 11.0 & 13.5 & 7.7 & 8.8 & 10.6 & 13.4 & 8.5 & 8.3 & \textbf{10.5} & 13.3 \\
		& & 45 & 7.2 & 7.6 & 10.7 & 12.6 & 7.6 & 7.9 & 11.0 & 13.1 & 8.3 & 8.8 & 11.1 & 13.7 & 7.8 & 8.9 & 11.0 & 13.4 & 8.5 & 8.5 & 10.9 & 13.3 \\
		& & 50 & 7.2 & 7.7 & 10.9 & 12.9 & 7.6 & 8.1 & 11.1 & 13.2 & 8.2 & 9.0 & 11.0 & 13.6 & 7.8 & 9.0 & 11.0 & 13.5 & 8.3 & 8.7 & 10.9 & 13.9 \\ \cline{2-23}
		& \multirow{10}{*}{\rotatebox{90}{Gaussian \acs{SVM}}} & 5 & 7.1 & 7.9 & 14.0 & 16.9 & 7.3 & 7.8 & 13.9 & 16.7 & 8.0 & 8.3 & 13.7 & 17.1 & 7.6 & 8.1 & 13.4 & 16.4 & 8.0 & 7.6 & 13.2 & 16.3 \\
		& & 10 & 6.4 & 6.8 & 13.3 & 15.8 & 6.9 & 6.9 & 13.3 & 15.7 & 7.4 & 7.7 & 12.9 & 15.7 & 7.3 & 7.9 & 12.9 & 15.4 & 7.5 & 7.5 & 12.9 & 15.3 \\
		& & 15 & \textbf{6.2} & 6.5 & 12.4 & 14.1 & 7.0 & 6.8 & 12.6 & 14.4 & 7.5 & 7.8 & 12.7 & 15.0 & 7.3 & 8.0 & 12.8 & 14.7 & 7.7 & 7.8 & 13.0 & 14.8 \\
		& & 20 & \textbf{6.2} & 6.3 & 11.9 & 13.9 & 6.9 & 7.0 & 12.0 & 14.1 & 7.5 & 8.1 & 12.5 & 15.0 & 7.6 & 8.1 & 12.5 & 14.7 & 7.8 & 8.1 & 13.0 & 14.8 \\
		& & 25 & 6.3 & \textbf{6.2} & 11.5 & 13.5 & 6.9 & 7.2 & 11.8 & 13.8 & 7.7 & 8.4 & 12.3 & 14.8 & 7.5 & 8.4 & 12.4 & 14.4 & 8.0 & 8.3 & 13.0 & 15.0 \\
		& & 30 & 6.3 & 6.3 & 11.1 & 13.0 & 7.1 & 7.5 & 11.8 & 13.9 & 7.9 & 8.6 & 12.4 & 15.0 & 7.6 & 8.6 & 12.4 & 14.6 & 8.2 & 8.5 & 13.0 & 15.0 \\
		& & 35 & 6.4 & \textbf{6.2} & 11.2 & 13.0 & 7.3 & 7.5 & 11.8 & 13.9 & 8.1 & 8.7 & 12.4 & 15.1 & 7.7 & 8.6 & 12.4 & 14.8 & 8.2 & 8.6 & 13.2 & 15.5 \\
		& & 40 & 6.5 & 6.3 & \textbf{11.0} & \textbf{12.9} & 7.4 & 7.7 & 11.9 & 14.0 & 8.1 & 8.8 & 12.5 & 15.2 & 7.8 & 8.7 & 12.4 & 14.8 & 8.3 & 8.7 & 13.3 & 15.4 \\
		& & 45 & 6.6 & 6.6 & 11.3 & 13.1 & 7.5 & 7.8 & 12.1 & 14.1 & 8.3 & 8.9 & 12.6 & 15.3 & 7.9 & 8.8 & 12.7 & 15.0 & 8.4 & 8.8 & 13.5 & 15.7 \\
		& & 50 & 6.6 & 6.7 & 11.2 & 13.0 & 7.5 & 8.0 & 12.2 & 14.3 & 8.4 & 9.1 & 12.8 & 15.5 & 7.9 & 9.0 & 12.8 & 15.2 & 8.4 & 8.9 & 13.7 & 15.8 \\ \hline
	\end{tabular}
\end{table*}
